# Supplementary material for: Finite/fixed-time Stabilization of Linear Systems with States Quantization
Source: arXiv:2309.01412 source file (2023-09-06)
Supplement: Supplementary file 1 [file appendix.tex]

\subsection*{Proof of Lemma \ref{lem:1}}
